# Supplementary material for: CNM: An Interpretable Complex-valued Network for Matching
Source: arXiv:1904.05298 source file (2019-04-10)
Supplement: Supplementary file 1 [file appendix.tex]

\begin{appendices}
\appendix
%Appendix A
\section{Preliminary}\label{Preliminary}
\subsection{Metric Space}
A \emph{metric space} is an ordered pair $(M,d)$ where $M$ is a set of samples while $d$ is a metric on $M$.
\begin{equation}
d : M \times M  \rightarrow \mathcal{R}
\end{equation}
A space could be a metric if and only if it holds these 4 rules, namely 	non-negativity,	identity of indiscernibles, symmetry and subadditivity (triangle inequality).
For example, $x,y,z \in M$, the non-negativity refers to
\begin{equation}
d(x,y) \ge 0
\end{equation}
the identity of indiscernibles refers to
\begin{equation}
d(x,y) =0 \Leftrightarrow  x=y
\label{indentity}
\end{equation}
the symmetry refers to
\begin{equation}
d(x,y) = d(y,x)
\end{equation}
the triangle inequality refers to
\begin{equation}
d(x,z) \ge d(x,y) + d(y,z)
\end{equation}
\section{Comments on so-called trace inner product}
\cite{sordoni2013modeling} uses the VN Divergence to compute the matching score between the query and document density matrix, since it could be asymmetric. It is expected to generate the query terms from document language model, and change the role of query and document. While in \cite{blacoe2013quantum} and \cite{zhang2018end}, both of these two tasks use a homogenous approach to build the density matrix. A symmetric metric distance is more reasonable. They adopt an alternative distance named so-called trace inner product.
\begin{equation}	
Similarity(\rho_a, \rho_b) = tr(\rho_a , \rho_b) = \epsilon - distance(\rho_a , \rho_b)
\end{equation}	

If we force this formula to follow the four rules of metric, we set $\epsilon$ as $tr(\rho_a \rho_a)$ to achieve the right-direction of  Eq.~\ref{indentity}.
\begin{equation}	
Distance(\rho_a , \rho_b) =  tr(\rho_a \rho_a) - tr(\rho_a  \rho_b)
\end{equation}	
Especially partly holding the the identity of indiscernibles. %If and only if $\rho_a == \rho_b$, we have the minimum value of the distance, namely 0. why ???
But it is an open question to proof the correctness of both identity of indiscernibles and non-negativity.
As mentioned by Prof. Melucci, we can not make sure that
\begin{equation}	
 tr(\rho_a \rho_a) \overset{?}> tr(\rho_a  \rho_b)
\end{equation}

Qiuchi demos  a counterexample for this in the case of $\mathcal{H}^2$.
For example, $\rho_a = \alpha  \ket{\phi_1} \bra{\phi_1}  +  (1-\alpha) \ket{\phi_2} \bra{\phi_2}$ and $\rho_a = \ket{\phi_1} \bra{\phi_1}$, $\ket{\phi_1}$ is orthogonal  to $\ket{\phi_2}$. We have

\begin{equation}	
\begin{aligned}
tr(\rho_a,\rho_a) -tr(\rho_a,\rho_b) &= \alpha ^2 + (1-\alpha  )^2 - \alpha  \\
&= 2 \alpha ^2 - 3 \alpha +1   \\
&= (\alpha-1)(2\alpha -1) \\
\end{aligned}
\end{equation}

The property for positive and negative would change if x ranges from  $[0,\frac{1}{2}]$ to  $[\frac{1}{2},1]$, thus it does not hold the identity of indiscernibles.

%
%Especially holding the the identity of indiscernibles. If and only if $\rho_a == \rho_b$, we have the minimum value of the distance, namely 0.

In addition, since the trace is invariant under cyclic permutations, i.e.,  $tr(ABCD) = tr(DABC) = tr(CDAB) =tr(BCDA)$. It naturally follow the symmetry.

We use simulation experiment to find some counterexamples to demonstrate that this does not hold the identity of indiscernibles and  the triangle inequality, in only a few cases.
However, we could not any effective proof about this.
\section{Linking to VSM for trace inner product}

Noting the following formula in \cite{zhang2018end}. It needs to be further explained.
\begin{equation}	
tr(\rho_a \rho_b) = \sum_{i,j} \lambda_i \lambda_j  \braket{r_i | r_j}^2
\label{vsm}
\end{equation}

This could be also explain with the Salton’s vector space model when the basis vectors are not orthogonal\cite{melucci2008basis}. Since the trace inner product has already ignored the probability property of density matrix. In other word, trace inner product treats density matrix as a normal matrix. If we reshape this matrix $\ket{\phi_i} \bra{\phi_i}$ into a longer vector $\ket{u_i} \in \mathcal{R}^{n^2}$,
\begin{equation}
\begin{aligned}	
\rho_a = \sum_i{p_i \ket{\phi_i} \bra{\phi_i}} =  \sum_i{p_i \ket{u_i} }\\
\rho_b = \sum_i{q_i \ket{\psi_i} \bra{\psi_i}} =   \sum_i{q_i \ket{v_i} }
\end{aligned}
\end{equation}
We can get the distance as follows
\begin{equation}	
vsm(\rho_a ,\rho_b) = \sum_{i,j} \lambda_i \lambda_j  \braket{u_i | v_j}^2
\end{equation}
which correspondings to Eq.~\ref{vsm}.
\section{ VN Divergence for Neural network}

Von-Neumann (VN) Divergence \cite{neumann1955mathematical} is usually used by measured the distance between two density matrices.
\begin{equation}
%\begin{aligned}	
 - \Delta_{VN} (\rho_a || \rho_b) = tr(\rho_a ( log \rho_a -log\rho_b)) \\
%\end{aligned}	
\end{equation}

log denotes a matrix logarithm, which means apply the classical logarithm to the matrix eigenvalues. if $\rho_a$  is fixed, the term $\rho_a log\rho_a$ can not change the ranking order and can be removed to the ranking score, as shown in \cite{sordoni2013modeling}.
\begin{equation}
 - \Delta_{VN} (\rho_a || \rho_b) \overset{rank}= tr(\rho_a log \rho_b)
\end{equation}

If we want to integrate the proposed distance/similaty metric into neural network, we should be sure that the function is differentiable and can be taken with the derivative in back propagation phrase. If the function is nondifferentiable, we can not train the model with in an end-2-end approach, or resort to expensive reinforce learning(it is not expected).

In neural network, the matching pair might be dual. In other words, the input of both side should be homogenous. Thus a symmetric metric is reasonable to be adopted. More importantly, the matching function should not be costly, in order to reduce the time consuming.

In this section, we will discuss the possibility of the VN-divergence in neural network. Firstly it is easy to make this metric symmetric like
\begin{equation}
\begin{aligned}	
sym-VN &= \frac{1}{2}(VN(\rho_a,\rho_b)+VN(\rho_b,\rho_a)) \\
 &=\frac{1}{2}tr(\rho_a ( log \rho_a -log\rho_b)) + tr(\rho_b ( log \rho_b -log\rho_a))
\end{aligned}
\end{equation}

The key concern is whether the log  matrix logarithm is differentiable or not.
\benyouqiuchi{It seems that it could be differentiable, and we should check whether it could be easily implemented by some Deep learning framework likeTensorflow/Pytorch/Keras. Moreover, the log  matrix logarithm is costly, due to that its time complexity is about $O(n^3)$  }

In addition, if remove the log  matrix logarithm with only adopting $tr(\rho_a,\rho_b)$ as metric. We might consider whether map $g( tr(\rho_a,\rho_b), VN(\rho_a,\rho_b)$ is monotonically increasing/decreasing, while g is functional mapping.
 \begin{equation}	
g : \mathcal{F} (\rho_a,\rho_b) \overset{g} \longrightarrow  \mathcal{F}' (\rho_a,\rho_b)
\end{equation}

\benyouqiuchi{The answer remains still open for us, we might guess that $g( tr(\rho_a,\rho_b), VN(\rho_a,\rho_b)$ is not monotonically increasing or decreasing either.}

\section{Theoretical comparison }
\begin{table*}[h]
\scriptsize
\begin{tabular}{lcccccc}
\hline
metric &  non-negativity & identity & symmetry & triangle inequality&differentiability  & computing complexity\\
\hline
trace inner product& - &- &-&-&+& $O(n^3)$\\
VN divergence& +&+&-&-&?&$O(n^3)$\\
sym-VN& +& +&+&-&?&$O(n^3)$\\
Fidelity& +& + &+&-&?&$O(n^3)$\\
square root of Fidelity & +& + &+&+&?&$O(n^3)$\\
partial POVM&+ &+ &+&?&+&$O(n^3)$\\

\hline
\end{tabular}
\end{table*}
$+$ means holding while $-$ means not holding. $?$ is noted that we are not clear about it. The results need be reviewed.
\section{A further understand of density matrix in statistic perspective.}

\subsection{Conclusions}
\subsection{References}
Generated by bibtex from your \texttt{.bib} file.  Run latex,
then bibtex, then latex twice (to resolve references)
to create the \texttt{.bbl} file.  Insert that \texttt{.bbl}
file into the \texttt{.tex} source file and comment out
the command \texttt{{\char'134}thebibliography}.
% This next section command marks the start of
% Appendix B, and does not continue the present hierarchy
\end{appendices}
